# Supplementary material for: Physics-inspired analysis of the two-class income distribution in the USA in 1983-2018
Source: arXiv:2110.03140 ancillary file (2022-01-05)
Supplement: Supplementary file 1 [file supplement.pdf]

# Supplemental Material for "Physics-inspired analysis of the two-class income distribution in the USA in 1983–2018" (arXiv:2110.03140)

Danial Ludwig and Victor M. Yakovenko
*JQI, Department of Physics, University of Maryland, College Park, MD 20742, USA*
(Dated: November 28, 2021)

## I. DATA SOURCE

The IRS Publication 1304 reports statistics based on a stratified sample of individual income tax returns from a given year [1]. The income and tax data used in this paper comes from Publication 1304, Table 1.1: "Selected Income and Tax Items, by Size and Accumulated Size of Adjusted Gross Income". Adjusted gross income (AGI) is defined as total income (e.g. salaries and wages, net capital gain, business income) minus statutory adjustments (e.g. self-employment expenses, retirement contributions, student loan interest), which are commonly known as "above-the-line deductions". Table 1.1 reports estimates of the number of tax returns, the total adjusted gross income less deficit, and total income tax revenue that falls in fixed AGI bins. We use the first of these to construct the cumulative distribution function (CDF), and the second and third to construct the income and tax Lorenz curves.

One alteration to the original data is made: Tax returns with zero or negative AGI are dropped before constructing the CDF and Lorenz curves. This corresponds to the "No AGI" bin from Table 1.1, in which 1-2% of the total number of tax returns fall each year. The choice to drop these returns is consistent with the methodology of the World Bank in their global poverty estimates [2]. Most returns with no AGI report net losses in areas such as self-owned businesses or the sale of capital assets, and are therefore seen as unlikely to accurately reflect the welfare of an individual.

Inflation data is also used to construct Figure 3. We use the annual average of the Consumer Price Index for all Urban consumers (CPI-U) as published by the Bureau of Labor Statistics. The CPI-U is the most widely used CPI and represents the expenditure patterns of 93% of the US population [3].

## II. DATA ANALYSIS

### A. Parameters $T$, $\alpha$, $r_*$, and $f_p$

The main challenge in analyzing the IRS distributional data is to fit samples from a smooth CDF to the piecewise function described in Eq. (3.1) of the paper:

$$C_{\rm add}(r) = e^{-r/T}, \quad C_{\rm mult}(r) \propto \frac{1}{r^\alpha},$$

where $T$ is the income temperature and $\alpha$ is the Pareto exponent. The cutoff point $r_*$ between the lower and upper classes is defined as the income at which $C_{\rm add}(r)$ and $C_{\rm mult}(r)$ intersect, so some other criterion must be used to determine which points to fit to which function. Fitting fewer points may increase the random uncertainties in the estimates of $T$ and $\alpha$, but may also reduce systematic uncertainties that arise from including points that lie in the interpolating region of the distribution.

The fitting procedure for $T$ is as follows. We first interpolate the CDF via Matlab's PCHIP (piecewise cubic Hermite interpolating polynomial) algorithm in log-linear scale. The PCHIP algorithm produces a $C^1$ interpolation that preserves monotonicity [4] and is therefore the best commonly-available procedure to apply to both CDFs and Lorenz curves. We then estimate $T$ by finding the income at which the interpolated CDF drops to $1/e$. Finally, we find $T$ by performing a linear least-squares fit in log-linear scale to all points with income less than the estimated $T$. We use a cutoff proportional to $T$, because it represents a natural income scale for the distribution, as shown in Figure 1 in the paper. Figure 3 implies that choosing a cutoff proportional to the median income $r_{\rm med}$ or the CPI-U would give somewhat similar results. We chose $T$ specifically as the cutoff because larger multiples produce values of $T$ that are skewed by deviations away from exponential. Using $1.5T$ as the cutoff, for example, includes points that deviate below exponential for 1980–1995, thereby underestimating $T$, and points that deviate above exponential for 2005–2018, thereby overestimating $T$.

Because the IRS reports fewer income bins at the higher end of the income distribution, $\alpha$ is more sensitive than $T$ to varying the number of points included in the fit. Examining the CDF in log-log scale reveals that the last three points ($200k, $500k, and $1M) reported by the IRS from 1983–1990 fall along a straight line. However, inflation implies that these constant nominal income bins effectively sample the CDF at decreasing real income levels over time. This can be seen in Figure 1, where the data points of each year are slightly to the left of those from the previous year. The incremental shift due to inflation causes the $200k point to move into the interpolating region during the mid-1990s. Then, starting in 2000, the IRS began reporting four additional bins at the high end of the distribution: $1.5M, $2M, $5M, and $10M. We find $\alpha$ by performing a linear least-

squares fit in log-log scale on the last three points from 1983–1992, the last two points from 1993–1999, and the last six points from 2000–2018. These three different regions of $\alpha$ are marked in Figure 4 by a dashed line connecting 1992–1993 and 1999–2000.

The crossover income dividing the upper and lower classes, $r_*$, and the fraction of population in the upper class, $f_p$, are then obtained by finding the intersection of $C_{\text{add}}$ and $C_{\text{mult}}$ for each year. As $r_*$ is dependent on $\alpha$, dashed lines are put in its plot in Figure 4 as well.

### B. Parameters $r_0$ and $\alpha_i$

For the last 10 years in the data set, 2009–2018, we also fit an interpolated form of the probability distribution, given by Eq. (2.11) in the paper:

$$P_{\text{int}}(r) = c\frac{e^{-(r_0/T)\arctan(r/r_0)}}{[1+(r/r_0)^2]^{(1+\alpha_i)/2}}.$$

For each year, we fix the value of $T$ as obtained in Part A, numerically integrate Eq. (2.11), and extract the Pareto exponent $\alpha_i$ and crossover income level $r_0$ simultaneously by performing a least-squares fit of the CDF data in log-linear scale. $T$ is kept separate, because fitting all three parameters together causes the procedure to be unstable.

### C. Parameters $f_r$, $f_t$, $G$, and $G_{\text{tax}}$

The fraction of income earned by the upper class, $f_r$, and fraction of tax revenue from the upper class, $f_t$, are calculated from $f_p$. The Matlab PCHIP algorithm is applied to the income and tax Lorenz curves, and these interpolants are evaluated at $1-f_p$ to get $1-f_r$ and $1-f_t$, as shown in Figure 7. The interpolants are also used to calculate the Gini coefficient for the income Lorenz curve, $G$, and the tax Lorenz curve, $G_{\text{tax}}$. The Gini coefficient is defined as twice the area between the Lorenz curve and the diagonal line of equality, so $G$ and $G_{tax}$ are obtained from integrating the interpolated income and tax Lorenz curves.

### D. Parameter $f_L$

We restrict consideration to the years with Gini coefficient greater than 0.5, where the theoretical formula $G = (1+f_L)/2$ can be applied. Fitting $f_L$ poses a challenge similar to that faced when fitting $T$. Some criterion must be used to decide which points along the income Lorenz curve to fit to the rescaled exponential distribution for the lower class, Eq. (3.6):

$$y = (1-f_L)[x + (1-x)\ln(1-x)].$$

Choosing either too few points or too many points skews the fit curve up, towards the line of equality, thus underestimating the value of $f_L$. Therefore, for each year we choose to fit the number of points that maximizes $f_L$. This choice amounts to dropping the last 3 or 4 points at the high end of the distribution from 1988–1999 and the last 7 or 8 points from 2000–2018.


[1] Internal Revenue Service (IRS), Statistics of Income (SOI) research division, "Individual Income Tax Returns", Publication 1304, `https://www.irs.gov/statistics/soi-tax-stats-individual-income-tax-returns-complete-report-publication-1304`

[2] The World Bank, Development Economics Division, "PovcalNet Methodology", `http://iresearch.worldbank.org/PovcalNet/methodology.aspx#`

[3] Bureau of Labor Statistics (BLS), "Handbook of Methods: Consumer Price Index", `https://www.bls.gov/opub/hom/cpi/concepts.htm`

[4] F. N. Fritsch and R. E. Carlson, "Monotone cubic piecewise interpolation", SIAM Journal on Numerical Analysis **17** (1980) 238, `https://doi.org/10.1137/0722023`
